# Supplementary material for: Definition of a scoring parameter to identify low-dimensional materials components
Source: arXiv:1808.02114 ancillary file (2019-03-19)
Supplement: Supplementary file 1 [file SI.pdf]

# 1 Density functional theory calculations

We have performed DFT calculations using the atomic simulation environment (ASE) [1, 8] and the GPAW [9, 5] electronic structure code and present below the density of states for 10 selected materials. The title in the figures gives, besides the chemical formula and ICSD number, the exchange-correlation functional used and the magnetic state [non-magnetic (NM), ferromagnetic (FM), and antiferromagnetic (AFM)]. In general we only present electronic spectrums for the lowest energy magnetic state for each exchange-correlation functional.

Calculations where performed for the experimental structures taken from ICSD database and using three different exchange-correlation functionals: PBE [10], PBE with a Hubbard U correction (PBE+U) [4], and the GLLB-SC [7] functional. PBE+U was chosen since some of the compounds contains transition metal atoms for which the Hubbard U correction can change the electronic structure qualitatively, i.e. from a metal to a semi-conductor. The Hubbard U correction was applied to the highest lying d-orbitals of transition metals and, for simplicity, a value of 4 eV for U was used irrespective of the atomic species. The GLLB-SC functional was chosen since it tends to give quasiparticle band gaps in better agreement with experiments than PBE [7, 3, 6]. Note that only non-magnetic calculations where done with the GLLB-SC functional.

The calculations where performed using a plane wave basis set with a cutoff energy of 800 eV, a Fermi-Dirac smearing of the occupations of the Kohn-Sham wave functions of 0.01 eV, and the Brillouin zone was sampled using a uniform grid with a $k$-point density of 12 1/Å$^{-1}$. To describe the ions, the projector augmented wave (PAW) method [2] was used with the GPAW atomic setups with version number 0.9.20000 (https://wiki.fysik.dtu.dk/gpaw/setups/setups.html).

To calculate the density of states projected onto the different dimensionality components of the compounds the (atom localized) projector functions in the PAW method where used to project the Kohn-Sham states onto. The projected density of states is performed without taking spin-orbit coupling effects into account.

# References


[1] S R Bahn and Karsten Wedel Jacobsen. An object-oriented scripting interface to a legacy electronic structure code. *Comput. Sci. Eng.*, 4(3):56–66, May 2002.

[2] P. E. Blöchl. Projector augmented-wave method. *Phys. Rev. B*, 50:17953–17979, Dec 1994.

[3] Ivano E. Castelli, Thomas Olsen, Soumendu Datta, David D. Landis, Soren Dahl, Kristian S. Thygesen, and Karsten W. Jacobsen. Computational screening of perovskite metal oxides for optimal solar light capture. *Energy Environ. Sci.*, 5:5814–5819, 2012.

[4] S. L. Dudarev, G. A. Botton, S. Y. Savrasov, C. J. Humphreys, and A. P. Sutton. Electron-energy-loss spectra and the structural stability of nickel oxide: An lsda+u study. *Phys. Rev. B*, 57:1505–1509, Jan 1998.

[5] Jussi Enkovaara, C Rostgaard, J J Mortensen, J Chen, M Dułak, L Ferrighi, J Gavnholt, C Glinsvad, V Haikola, H A Hansen, H H Kristoffersen, M. Kuisma, A H Larsen, L Lehtovaara, M Ljungberg, O Lopez-Acevedo, P G Moses, J Ojanen, T Olsen, Vivien Petzold, N A Romero, J Stausholm-Møller, M Strange, G A Tritsaris, M Vanin, Michael Walter, Bjørk Hammer, H. Hakkinen, G K H Madsen, R M Nieminen, Jens K Nørskov, M Puska, T T Rantala, J Schiøtz, Kristian Sommer Thygesen, and Karsten Wedel Jacobsen. Electronic structure calculations with GPAW: a real-space implementation of the projector augmented-wave method. *J. Phys. Condens. Matter*, 22(2):3202, June 2010.

[6] Sten Haastrup, Mikkel Strange, Mohnish Pandey, Thorsten Deilmann, Per S Schmidt, Nicki F Hinsche, Morten N Gjerding, Daniele Torelli, Peter M Larsen, Anders C Riis-Jensen, Jakob Gath, Karsten W Jacobsen, Jens Jørgen Mortensen, Thomas Olsen, and Kristian S Thygesen. The Computational 2D Materials Database: high-throughput modeling and discovery of atomically thin crystals. *2D Materials*, 5(4):042002, 2018.

[7] M. Kuisma, J. Ojanen, J. Enkovaara, and T. T. Rantala. Kohn-sham potential with discontinuity for band gap materials. *Phys. Rev. B*, 82:115106, Sep 2010.

[8] Ask Larsen, Jens Mortensen, Jakob Blomqvist, Ivano Eligio Castelli, Rune Christensen, Marcin Dulak, Jesper Friis, Michael Groves, Bjørk Hammer, Cory Hargus, Eric Hermes, Paul Jennings, Peter Jensen, James Kermode, John Kitchin, Esben Kolsbjerg, Joseph Kubal, Kristen Kaasbjerg, Steen Lysgaard, Jon Maronsson, Tristan Maxson, Thomas Olsen, Lars Pastewka, Andrew Peterson, Carsten Rostgaard, Jakob Schiøtz, Ole Schütt, Mikkel Strange, Kristian Sommer Thygesen, Tejs Vegge, Lasse Vilhelmsen, Michael Walter, Zhenhua Zeng, and Karsten Wedel Jacobsen. The Atomic Simulation Environment - A Python library for working with atoms. *J. Phys. Condens. Matter*, 29(27):273002, Mar 2017.

[9] J J Mortensen, L B Hansen, and Karsten Wedel Jacobsen. Real-space grid implementation of the projector augmented wave method. *Phys. Rev. B*, 71(3):35109, Jan 2005.

[10] John P. Perdew, Kieron Burke, and Matthias Ernzerhof. Generalized gradient approximation made simple. *Phys. Rev. Lett.*, 77:3865–3868, Oct 1996.

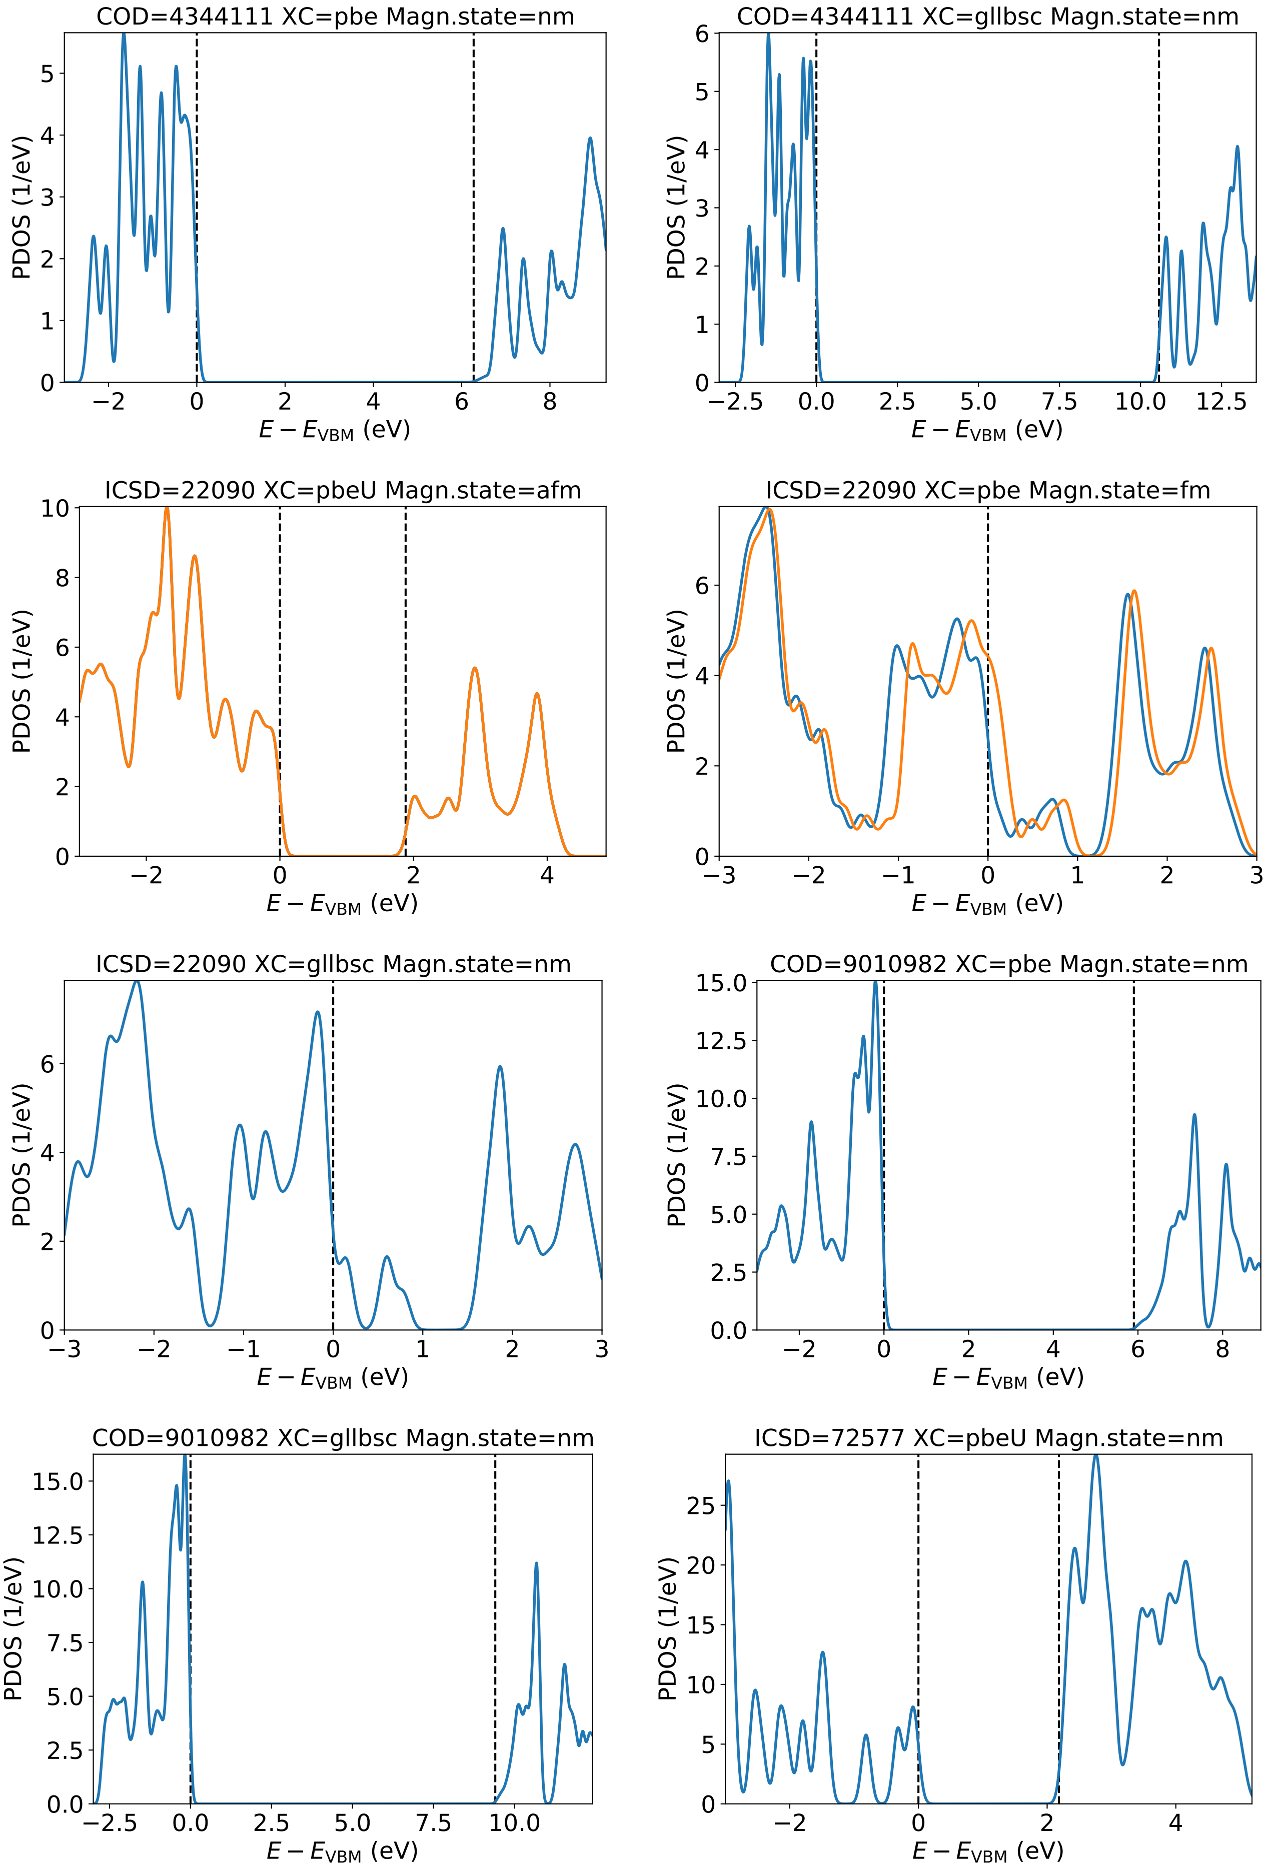
COD=4344111 XC=pbe Magn.state=nm
COD=4344111 XC=gllbsc Magn.state=nm
ICSD=22090 XC=pbeU Magn.state=afm
ICSD=22090 XC=pbe Magn.state=fm
ICSD=22090 XC=gllbsc Magn.state=nm
COD=9010982 XC=pbe Magn.state=nm
COD=9010982 XC=gllbsc Magn.state=nm
ICSD=72577 XC=pbeU Magn.state=nm
PDOS (1/eV)
$E - E_{\mathrm{VBM}}$ (eV)

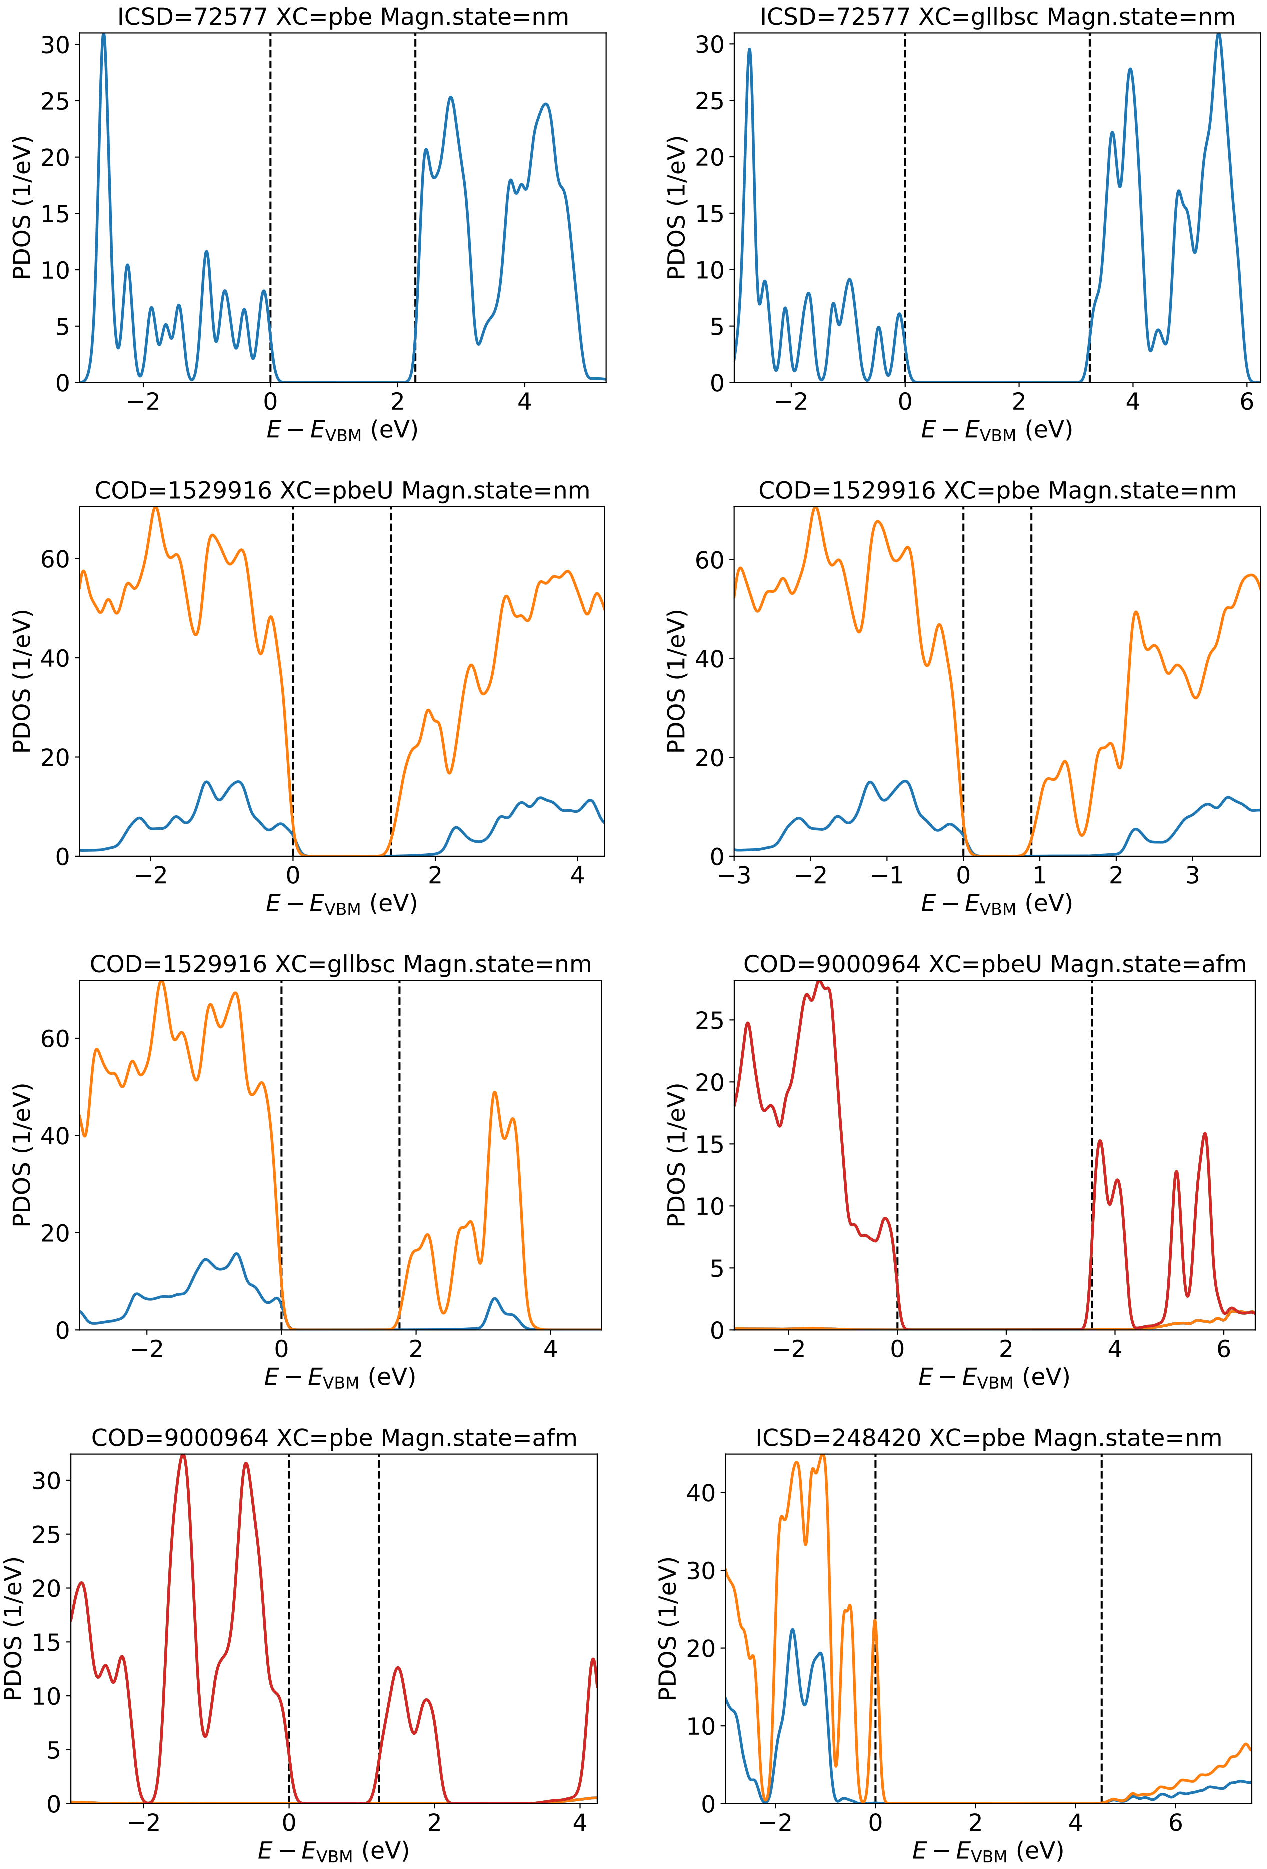
ICSD=72577 XC=pbe Magn.state=nm
ICSD=72577 XC=gllbsc Magn.state=nm
COD=1529916 XC=pbeU Magn.state=nm
COD=1529916 XC=pbe Magn.state=nm
COD=1529916 XC=gllbsc Magn.state=nm
COD=9000964 XC=pbeU Magn.state=afm
COD=9000964 XC=pbe Magn.state=afm
ICSD=248420 XC=pbe Magn.state=nm
PDOS (1/eV)
$E - E_{\mathrm{VBM}}$ (eV)

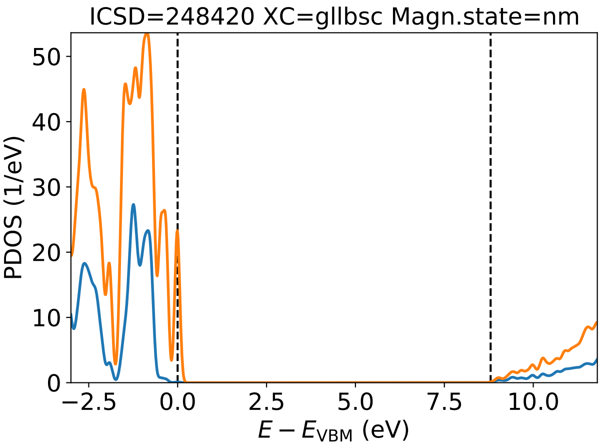
ICSD=248420 XC=gllbsc Magn.state=nm
PDOS (1/eV)
$E - E_{\mathrm{VBM}}$ (eV)

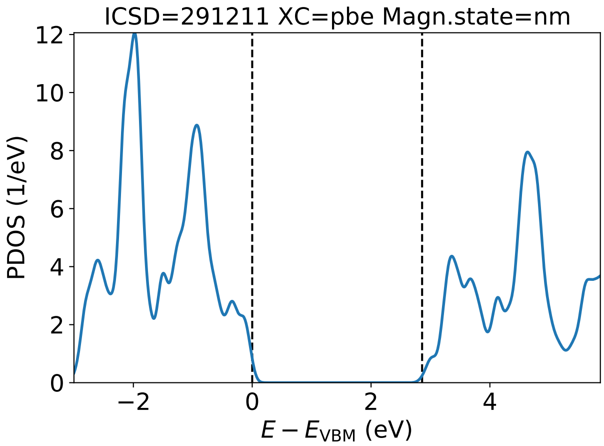
ICSD=291211 XC=pbe Magn.state=nm
PDOS (1/eV)
$E - E_{\mathrm{VBM}}$ (eV)

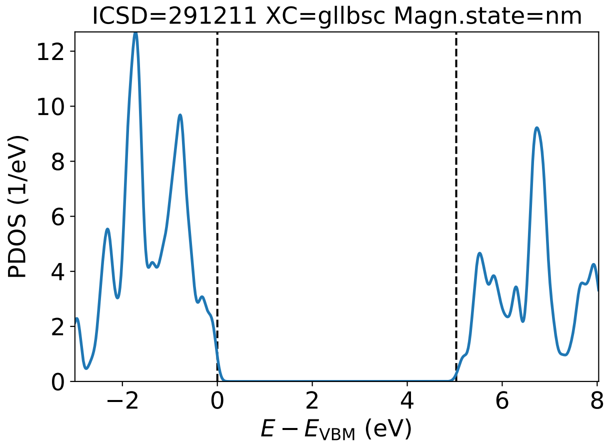
ICSD=291211 XC=gllbsc Magn.state=nm
PDOS (1/eV)
$E - E_{\mathrm{VBM}}$ (eV)

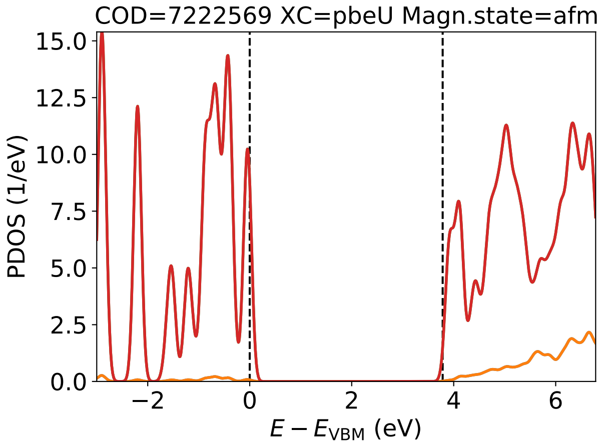
COD=7222569 XC=pbeU Magn.state=afm
PDOS (1/eV)
$E - E_{\mathrm{VBM}}$ (eV)

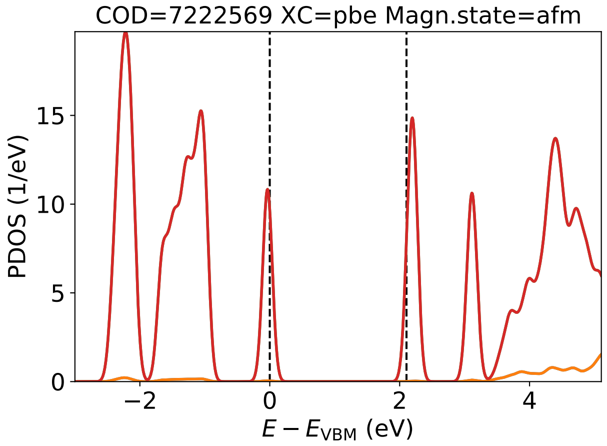
COD=7222569 XC=pbe Magn.state=afm
PDOS (1/eV)
$E - E_{\mathrm{VBM}}$ (eV)

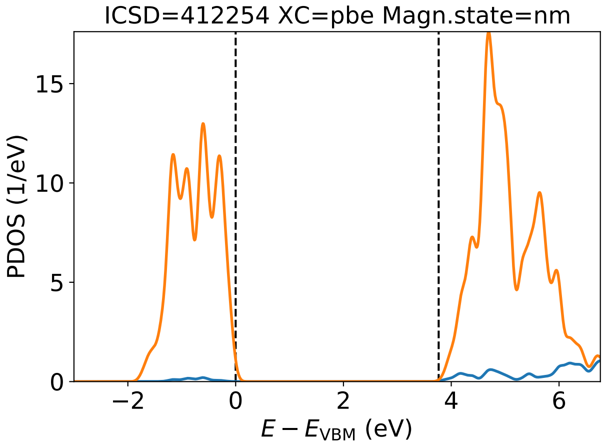
ICSD=412254 XC=pbe Magn.state=nm
PDOS (1/eV)
$E - E_{\mathrm{VBM}}$ (eV)

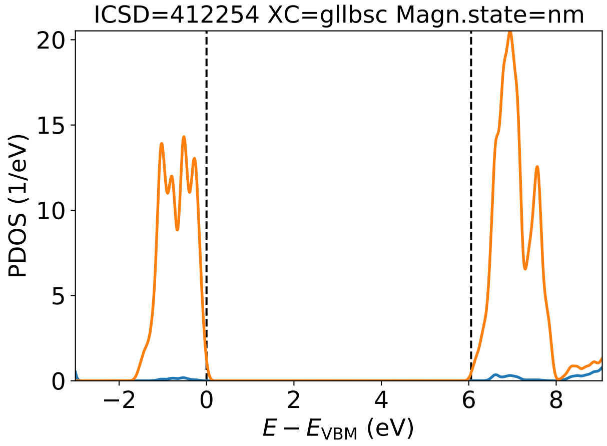
ICSD=412254 XC=gllbsc Magn.state=nm
PDOS (1/eV)
$E - E_{\mathrm{VBM}}$ (eV)
